# Supplementary material for: Testing Calibration in Nearly-Linear Time
Source: arXiv:2402.13187 source file (2024-06-21)
Supplement: Supplementary file 1 [file appendix.tex]

\section{Smooth calibration using box-simplex games}\label{sec:smooth_appendix}

In this section, we provide our main result on approximating the smooth calibration of a distribution on $[0, 1] \times \{0, 1\}$. In Section~\ref{ssec:round_smooth}, we first develop a rounding procedure compatible with the smooth calibration linear program (in the sense of Definition~\ref{def:rounding}), when applied to an empirical distribution. We provide some discussion of a simpler variant of our rounding procedure in Section~\ref{ssec:sbase}.

Similar to Corollary \ref{cor:l_1}, we also have the following analog for a variant of $\ell_\infty$ regression.

\begin{corollary}\label{cor:l_inf}
Let $\ma \in \R^{n \times d}, b \in \R^n, c \in \R^d$, and $\eps > 0$. There is an algorithm which computes an $\eps$-approximate minimizer to $\min_{x \in [-1, 1]^d} c^\top x + \norm{\max\Par{\ma x - b, \0_n}}_\infty$, 
where the $\max$ operation is entrywise, in time
\[O\left(\nnz(\ma)\cdot\frac{\norm{\ma}_{\infty \to \infty}\log n}{\eps}\right).\]
\end{corollary}
\begin{proof}
First, observe that we can rewrite the given objective as
\[\min_{x \in [-1, 1]^d} \max_{y \in \Delta^{n + 1}} c^\top x + y^\top(\tma x - \tb),\]
where $\tma \in \R^{(n + 1) \times d}$ appends an extra all-zeroes row to $\ma$, and $\tb \in \R^{n + 1}$ appends an extra zero to $b$. Namely, if $\ma x - b \le \0_n$ entrywise, we have $y^\top (\tma x - \tb) = 0 = \norm{\max(\ma x - b, \0_n)}_\infty$, and otherwise $y^\top(\tma x - \tb)$ chooses the largest entry of $\ma x - b$. The conclusion follows from Proposition~\ref{prop:box_simplex}, using 
\[\norms{\tma}_{\infty \to \infty} = \norm{\ma}_{\infty \to \infty} = \norms{\ma^\top}_{1 \to 1}.\]
\end{proof}

\subsection{Rounding for empirical smooth calibration}\label{ssec:round_smooth}

In this section, we develop an efficient algorithm for computing the smooth calibration error of an empirical distribution. Specifically, throughout the section, we fix a dataset under consideration,
\[\hcD_n \defeq \Brace{(v_i, y_i)}_{i \in [n]} \subset [0, 1] \times \{0, 1\},\]
and the corresponding empirical distribution (which, in an abuse of notation, we also denote $\hcD_n$), i.e.\ we use $(v, y) \sim \hcD_n$ to mean that $(v, y) = (v_i, y_i)$ with probability $\frac 1 n$ for each $i \in [n]$. We also assume without loss of generality that the $\{v_i\}_{i \in [n]}$ are in sorted order, so $0 \le v_1 \le \ldots \le v_n \le 1$. Recalling Definition~\ref{def:smooth}, the associated empirical smooth calibration linear program is
\begin{equation}\label{eq:smce_empirical_appendix}
\begin{aligned}
\smce(\hcD_n) \defeq \max_{\substack{x \in \xset \\ \ma x \le b} } c^\top x, \text{ where } \xset &\defeq [-1, 1]^n, \\
c_i &\defeq \frac 1 n (y_i - v_i) \text{ for all } i \in [n], \\
b_{(i, j, +)} = b_{(i, j, -)} &\defeq v_j - v_i \text{ for all } (i, j) \in [n] \times [n] \text{ with } i < j, \\
\text{and } \ma_{(i, j, +):} &\defeq e_j - e_i, \\
\ma_{(i, j, -):} &\defeq e_i - e_j,\text{ for all } (i, j) \in [n] \times [n] \text{ with } i < j.
\end{aligned}\end{equation}
Here, $x_i$ represents the value $w(v_i)$. Because $x = \0_n$ is always feasible, the maximum $\inprod{c}{x}$ is nonnegative, so we can drop the absolute value in Definition~\ref{def:smooth}. Moreover, $\ma$ and $b$ have rows identified with $[2\binom{n}{2}]$, i.e.\ doubled pairs of sorted indices in $[n] \times [n]$, enforcing the Lipschitz constraints
\[\max(x_j - x_i, x_i - x_j)  \le v_j - v_i \text{ for all } (i, j) \in [n] \times [n] \text{ with } i < j.\]
Our solver for \eqref{eq:smce_empirical_appendix} goes through the machinery of Definition~\ref{def:rounding}; we design a $(\tma, \tb, \infty)$-inequality rounding procedure for $(\ma, b, c, \xset)$ in \eqref{eq:smce_empirical_appendix}. We let $\tma, \tb$ be carefully chosen subsets of the rows of $\ma, b$, with $O(n)$ rows. Before formally stating our choices of $\tma, \tb$, we give several helper lemmas.

 \begin{lemma}\label{lem:three points}
 Let $i, j, k \in [n]$ with $i < j < k$. Suppose that for $\Delta \ge 0$ and $v, x \in \R^n$ with $v_i \le v_j \le v_k$, 
 \[|x_i - x_j| \le v_j - v_i + \Delta,\; |x_i - x_k| \le v_k - v_i,\; |x_j - x_k| \le v_k - v_j + \Delta.\]
There is $y \in \R^n$ with $y_\ell = x_\ell$ for all $\ell \neq j$, $y_j \in [\min_{\ell \in [n]}x_\ell, \max_{\ell \in [n]} x_\ell]$, $|y_j - x_j| \le \Delta$, and    
\[|y_i - y_j| \le v_j - v_i,\; |y_i - y_k| \le v_k - v_i,\; |y_j - y_k| \le v_k - v_j.\]
 \end{lemma}
 \begin{proof}
We split into four cases, depending on which subset of the constraints $|x_i - x_j| \le v_j - v_i$ and $|x_j - x_k| \le v_k - v_j$ is false. In the first case, neither is false and returning $y \gets x$ suffices. 

In the second case, both are false, i.e.\
\begin{equation}\label{eq:case_2}v_j - v_i < |x_i - x_j| \le v_j - v_i + \Delta,\; v_k - v_j < |x_j - x_k| \le v_k - v_j + \Delta. \end{equation}
We claim that in this case, $x_j \le \min(x_i, x_k)$ or $x_j \ge \max(x_i, x_k)$. To see this, if $x_i \le x_j \le x_k$, then 
\begin{equation}\label{eq:both_not_tight}|x_j - x_i| + |x_k - x_j| = (x_j - x_i) + (x_k - x_j) = x_k - x_i \le v_k - v_i =  (v_j - v_i) + (v_k - v_j),\end{equation}
where we used $|x_i - x_k| \le v_k - v_i$, so we cannot have \eqref{eq:case_2} hold. Similarly, if $x_k \le x_j \le x_i$, this again contradicts \eqref{eq:case_2}. Now, we claim it suffices to choose $y = x$ coordinatewise except for $y_j$, defined by
\begin{equation}\label{eq:fix_both}y_j \gets x_j + \sign(x_i - x_j)\underbrace{\max\Par{\Par{|x_i - x_j| - (v_j - v_i)}, \Par{|x_k - x_j| - (v_k - v_j)}}}_{\defeq \zeta}.\end{equation}
In other words, we move $x_j$ towards the other two points by the larger of the two violation amounts in \eqref{eq:case_2}. To prove correctness of \eqref{eq:fix_both}, suppose $x_j \le \min(x_i, x_k)$ without loss of generality, so that $y_j = x_j + \zeta$ (the other case is symmetric by negating $x$). We first observe that
\begin{equation}\label{eq:y_still_bounded}\max(x_i, x_k) - x_j \ge \zeta \implies y_j \le \max(x_i, x_k).\end{equation}
Next, consider the subcase where $y_j \le \min(x_i, x_k)$. Then, $y_i - y_j = x_i - y_j = x_i-x_j -\zeta \leq v_j-v_i$ so the Lipschitz constraint on $(y_i, y_j)$ is enforced. We symmetrically have $y_k - y_j \le v_k - v_i$.

The other subcases are when $x_i\leq y_j \leq x_k$ or $x_k\leq y_j \leq x_i$, i.e.\ $y_j$ is in between $x_i$ and $x_k$. By the definition of $\zeta$, either $|y_j - x_i| = v_j - v_i$ or $|x_k - y_j| = v_k - v_j$ is a tight Lipschitz constraint, and in either case \eqref{eq:both_not_tight} shows that the other constraint is also enforced, since $|x_k - x_i| \le v_k - v_i$.
\iffalse
If $x_i\leq y_j \leq x_k$, we have either $x_k-y_j = x_k-x_j-\zeta = v_k-v_j$ or $y_j-x_i = x_j - x_i +\zeta = -(v_j-v_i)\geq 0$ which means $y_j-x_i = -v_j+v_i = 0 = v_j-v_i$. By the fact,
\[\abs{x_k-x_i} = x_k - y_j + y_j - x_i\leq v_k - v_i = v_k-v_j + v_j -v_i,\] the constraint left is fulfilled. 

It is similar when $x_k\leq y_j \leq x_i$. We have $x_i-x_k \leq v_k-v_i$ and either $x_i-y_j= x_i-x_j - \Delta = v_j-v_i$ or $y_j-x_k= x_j -x_k + \Delta = -(v_k-v_j)\geq 0$ which means $y_j-x_k = -v_k+v_j = 0 = v_k-v_j$. By the fact,
\[\abs{x_i-x_k} = x_i - y_j + y_j - x_k\leq v_k - v_i = v_k-v_j + v_j -v_i,\] the constraint left is fulfilled.
\fi

In the third case, we have
\begin{equation}\label{eq:case_3}v_j - v_i < |x_i - x_j| \le v_j - v_i + \Delta,\; |x_j - x_k| \le v_k - v_j.\end{equation}
We claim it suffices to choose
\begin{equation}\label{eq:fix_ij}y_j \gets x_j + \sign(x_i - x_j) \underbrace{(|x_i - x_j| - (v_j - v_i))}_{\defeq \zeta}.\end{equation}
Again assume without loss of generality that $x_j \le x_i$ and $y_j = x_j + \zeta$. By construction, $|y_j - x_i| = v_j - v_i$, so we need to check that $|y_j - x_k| \le v_k - v_j$. If originally $x_k \le x_j \le x_i$, then \eqref{eq:both_not_tight} shows $x_j - x_k \le (v_k - v_j) - \zeta$, so $|y_j - x_k| \le x_k - x_j + \zeta \le v_k - v_j$ as claimed. Otherwise, if $x_j \le x_k$, then \eqref{eq:y_still_bounded} shows $y_j \le x_i$. If $y_j \in [x_k, x_i]$, then $|y_j - x_i| = v_j - v_i$ and \eqref{eq:both_not_tight} show that $|y_j - x_k| \le v_k - v_j$ as well. Finally, if $y_j \le x_k$, then $0 \le x_k - y_j = x_k - x_j - \zeta \le v_k - v_j$, as desired.

In the fourth case, we have
\begin{equation}\label{eq:case_4}v_k - v_j < |x_k - x_j| \le v_k - v_j + \delta,\; |x_j - x_i| \le v_j - v_i.\end{equation}
We claim it suffices to choose
\begin{equation}\label{eq:fix_jk}y_j \gets x_j + \sign(x_k - x_j) \underbrace{(|x_k - x_j| - (v_k - v_j))}_{\defeq \zeta}.\end{equation}
The correctness analysis of \eqref{eq:fix_jk} proceeds symmetrically to the correctness analysis of \eqref{eq:fix_ij}. 

It is straightforward to check that in all cases, $|y_j - x_j| \le \Delta$, and $y_j$ stays in the range with endpoints $\min(x_i, x_j, x_k)$ and $\max(x_i, x_j, x_k)$, proving the other claimed conditions.
 \end{proof}

 Lemma~\ref{lem:three points} says that given three Lipschitz constraints induced by three coordinates of $v$, if the ``outer'' constraint is satisfied and the other two constraints are violated by $\le \Delta$, we can move the middle coordinate by $\le \Delta$ to fix all constraints. Moreover, it guarantees that if $x \in \xset = [-1, 1]^n$, then $y \in \xset$. We next observe that this procedure does not make adjacent constraints worse.

 \begin{lemma}\label{lem:protect_constraints_1}
 Let $i, j, h \in [n]$ with $i < j < h$. Suppose that for $\Delta \ge 0$ and $v, x \in \R^n$ with $v_i \le v_j \le v_h$,
 \[v_j - v_i \le |x_i - x_j| \le v_j - v_i + \Delta,\; |x_h - x_i| \le v_h - v_i + \Delta,\; |x_h - x_j| \le v_h - v_j + \Delta.\]
 Let $t = x_j - \sign(x_j - x_i) \cdot \zeta$ for $\zeta \in [0, |x_i - x_j| - (v_j - v_i)]$. Then, $|x_h - t| \le v_h - v_j + \Delta$.
 \end{lemma}
 \begin{proof}
The argument is symmetric in $x$ and $-x$, so assume without loss that $x_i \le x_j$ and 
\[t \in [x_i + (v_j - v_i), x_j].\]
If $x_h \le x_j$, then since $t \le x_j$, we have $|x_h - t| \le \max(|x_h - x_j|, |t - x_j|) \le \max(v_h - v_j + \Delta, \Delta) = v_h - v_j + \Delta$. Otherwise, if $x_h \ge x_j$, since $|x_h - t| = |x_h - x_j| + |x_j - t|$ in this case, we have
\[|x_h - t| = x_h - x_j + (x_j - x_i) - (v_j - v_i) \le v_h - v_j + \Delta, \]
which follows from $|x_h - x_i| = x_h - x_i \le v_h - v_i + \Delta$.
 \end{proof}

We remark that Lemma~\ref{lem:protect_constraints_1} applies exactly to moves of the form induced by Lemma~\ref{lem:three points}, regardless of the case of Lemma~\ref{lem:three points} we are in. We symmetrically have the following claim.

 \begin{lemma}\label{lem:protect_constraints_2}
 Let $h, j, k \in [n]$ with $h < j < k$. Suppose that for $\Delta \ge 0$ and $v, x \in \R^n$ with $v_h \le v_j \le v_k$,
 \[v_k - v_j \le |x_k - x_j| \le v_k - v_j + \Delta,\; |x_h - x_j| \le v_j - v_h + \Delta,\; |x_h - x_k| \le v_k - v_h + \Delta.\]
 Let $t = x_j - \sign(x_j - x_k) \cdot \zeta$ for $\zeta \in [0, |x_k - x_j| - (v_k - v_j)]$. Then, $|x_h - t| \le v_j - v_h + \Delta$.
 \end{lemma}

 Our rounding procedure design (parameterized by $\tma, \tb$) is motivated by the observations in Lemmas~\ref{lem:three points},~\ref{lem:protect_constraints_1}, and~\ref{lem:protect_constraints_2}. We fix three sets of index pairs in $[n] \times [n]$ as follows:
 \begin{equation}\label{eq:enforce_constraints_def}
 \begin{gathered}
 S \defeq \SB \cup \SL \cup \SR,\; L \defeq \lfloor\log_2(n - 1)\rfloor, \\
 \SB \defeq \Par{[n] \times [n]} \cap \bigcup_{\ell = 0}^L \Brace{\Par{(i - 1)2^\ell + 1, i2^\ell + 1} \mid i \in [2^{L - \ell}] },\\
 \SL \defeq \Par{[n] \times [n]} \cap \bigcup_{\ell = 1}^L \bigcup_{m = 0}^{\ell - 1} \Brace{\Par{(i - 1)2^\ell - 2^m + 1, i2^\ell + 1} \mid i \in [2^{L - \ell}] },\\
 \SR \defeq \Par{[n] \times [n]} \cap \bigcup_{\ell = 1}^L \bigcup_{m = 0}^{\ell - 1} \Brace{\Par{(i - 1)2^\ell + 1, i2^\ell + 2^m + 1} \mid i \in [2^{L - \ell}] }.\\
\end{gathered}
 \end{equation}
We also call the following set of indices in $S$ the \emph{$\ell^{\text{th}}$ layer of constraints}:
\begin{equation}\label{eq:layer_def}\begin{gathered}S_\ell \defeq \Par{\Par{[n] \times [n] } \cap \Brace{\Par{(i - 1)2^\ell + 1, i2^\ell + 1} \mid i \in [2^{L - \ell}] }}.\end{gathered}\end{equation}
In other words, for each $0 \le \ell \le L$, the $\ell^{\text{th}}$ layer of constraints is entirely due to $\SB$, and consists of index pairs in $[n] \times [n]$ spaced $2^\ell$ coordinates apart. There is a corresponding set of constraints due to $\SL$ which extends the $\ell^{\text{th}}$ layer of constraints, and consists of index pairs in $[n] \times [n]$ spaced $2^\ell + 2^m$ coordinates apart for each $0 \le m \le \ell - 1$, offset by $2^\ell$ coordinates each, where the left endpoint is extended $2^m$ beyond the corresponding constraint in $\SB$. We define $\SR$ symmetrically, extending right endpoints of intervals in $\SB$ by $2^m$ instead.

Our rounding procedure fixes Lipschitz constraints one layer at a time using Lemma~\ref{lem:three points}. We use Lemma~\ref{lem:protect_constraints_1} to make sure that fixing a higher layer does not worsen the violation of any lower layer, by using adjacent constraints in $\SR$ to protect the lower layer. Similarly, we use Lemma~\ref{lem:protect_constraints_2} to protect lower layers using adjacent constraints in $\SL$. This also explains our inclusion of the constraints $\SL$, $\SR$. For completeness, we give a discussion in Section~\ref{ssec:sbase} on why using only $\SB$ would result in losing a logarithmic factor in the rounding guarantee, yielding a similar loss in the runtime.

For example, if $n = 9$, so $L = 3$, $S$ defined in \eqref{eq:enforce_constraints_def} consists of the pairs
 \begin{gather*}
\SB = \Brace{(i, i + 1) \mid i \in [8]} \cup \Brace{(2i - 1, 2i + 1) \mid i \in [4]} \cup \Brace{(4i - 3, 4i + 1) \mid i \in [2]} \cup \Brace{(1, 9)}, \\
\SL = \Brace{(2i - 2, 2i + 1) \mid 2 \le i \le 4} \cup \Brace{(4, 9)} \cup \Brace{(3, 9)}, \\
\SR = \Brace{(2i - 1, 2i + 2) \mid i \in [3]} \cup \Brace{(1, 6)} \cup \Brace{(1, 7)}.
 \end{gather*}
We let $\tma$, $\tb$ be scaled row subsets of $\ma$, $b$ corresponding to $S$, i.e.\ following notation in \eqref{eq:smce_empirical_appendix}, \eqref{eq:enforce_constraints_def},
\begin{equation}\label{eq:round_def_smooth}\begin{aligned}
\tma \in \R^{2|S| \times n} \text{ has } \tma_{(s, +):} \defeq \ma_{(s, +):},\;\tma_{(s, -):} \defeq \ma_{(s, -):}  \text{ for all } s \in S,\; \\
\tb \in \R^{2|S|} \text{ has } \tb_{(s, +)} \defeq b_{(s, +)},\;  \tb_{(s, -)} \defeq b_{(s, -)}\text{ for all } s \in S.
\end{aligned}\end{equation}

We next show how to recursively apply Lemma~\ref{lem:three points} to show there exists an efficient $(\tma, \tb, \infty)$-inequality rounding procedure for $(\ma, b, c, \xset)$, recalling the definition of rounding procedures in Definition~\ref{def:rounding}. We begin by observing that it suffices to enforce the $0^{\text{th}}$ layer of constraints in $S$ to show feasibility.

We can now state and analyze our rounding procedure.

\begin{lemma}\label{lem:round_def_smooth}
Let $(\ma, b, c, \xset)$ be defined as in \eqref{eq:smce_empirical_appendix}, and let $(\tma, \tb)$ be defined as in \eqref{eq:enforce_constraints_def}, \eqref{eq:round_def_smooth}. There exists $\Round$, a $(\tma, \tb, \infty)$-inequality rounding procedure for $(\ma, b, c, \xset)$ running in $O(n)$ time.
\end{lemma}
\begin{proof}
For a fixed $x \in \xset$, let
\[\Delta \defeq \norm{\max\Par{\tma x - \tb, \0_{2|S|}}}_\infty,\]
so that $\Delta$ is the maximum violation of any Lipschitz constraint in $S$ at the start of the algorithm. We claim we can produce $x' = \Round(x) \in \xset$ with $\ma x' \le b$ (i.e.\ $x'$ satisfies all of the Lipschitz constraints in $[n] \times [n]$), such that $\norm{x - x'}_\infty \le \Delta$. This implies $\Round$ is a $(\tma, \tb, \infty)$-inequality rounding procedure as desired, because \eqref{eq:uncon_ineq_lp} then follows from $c \in [-\frac 1 n, \frac 1 n]^n \implies \|c\|_1 \le 1$, and
\[c^\top(x' - x) \le \norm{c}_1\norm{x' - x}_\infty \le \Delta = \norm{\max\Par{\tma x - \tb, \0_{2|S|}}}_\infty. \]

Next, we show how to produce $x' \in \xset$ satisfying $\ma x' \le b$ and $\norm{x - x'}_\infty \le \Delta$. Without loss of generality, let $n = 2^L + 1$; otherwise, we create $O(n)$ additional coordinates of $x$ and $v$, all equal to $x_n$ and $v_n$. We inductively apply Lemma~\ref{lem:three points} to each layer of constraints $0 \le \ell \le L$, starting from $\ell \gets L$ and $x^{(L + 1)} \gets x$. Each round of the algorithm corresponds to a single layer $\ell$, takes as input a point $x^{(\ell + 1)} \in \xset$, and modifies it to produce $x^{(\ell)} \in \xset$ as output. At the end of round $\ell$ (and therefore the start of $\ell - 1$), we maintain the following invariants on $x^{(\ell)}$.
\begin{enumerate}
    \item Every Lipschitz constraint $s$ in the $\ell^{\text{th}}$ layer holds, i.e.\ $\max(\ma_{(s, +):} x, \ma_{(s, -):} x) \le b_{(s, +)}$. \label{item:row_fixed}
    \item $\max(\ma_{(s, +):} x - b_{(s, +)}, \ma_{(s, -):} x - b_{(s, +)}) \le \Delta$ for all $s \in \SB$.\label{item:lower_constraints_ok}
    \item $\norms{x^{(\ell)} - x^{(\ell + 1)}}_\infty \le \Delta$.\label{item:inf_bound}
    \item Only coordinates of the form $j = i2^\ell + 1$ for odd $i \in \Z_{\ge 0}$ have $x^{(\ell + 1)}_j \neq x^{(\ell)}_j$. \label{item:sparse_move}
\end{enumerate}
Suppose for induction that Items~\ref{item:row_fixed},~\ref{item:lower_constraints_ok},~\ref{item:inf_bound}, and~\ref{item:sparse_move} all hold for all rounds in $[\ell, L]$, and consider the $(\ell - 1)^{\text{th}}$ round. We apply Lemma~\ref{lem:three points} to each $(\ell - 1)^{\text{th}}$ layer constraint, where the maximum violation of any constraint is $\Delta$ due to Item~\ref{item:lower_constraints_ok} from the previous round. By construction, Lemma~\ref{lem:three points} preserves Items~\ref{item:inf_bound} and~\ref{item:sparse_move}, and enforces Item~\ref{item:row_fixed} after completion. We are only left with Item~\ref{item:lower_constraints_ok}. To see that this is true, note that for each $m^{\text{th}}$ level constraint for $m < \ell - 1$, it can share an endpoint with at most one $(\ell - 1)^{\text{th}}$ level constraint; if it shares no endpoints, correctness of Item~\ref{item:lower_constraints_ok} clearly still holds. If it shares one endpoint, depending on whether the endpoint is on the left or the right of the $m^{\text{th}}$ level constraint, we use Lemma~\ref{lem:protect_constraints_1} or~\ref{lem:protect_constraints_2}, as well as existence of the relevant constraint in $\SL$ or $\SR$, to ensure that Item~\ref{item:lower_constraints_ok} holds after applying Lemma~\ref{lem:three points}. Finally, at the end of the algorithm, each coordinate has moved at most once, and by at most $\Delta$, via Items~\ref{item:inf_bound} and~\ref{item:sparse_move}. Because all the $0^{\text{th}}$-layer constraints hold by Item~\ref{item:row_fixed}, we have feasibility of $x^{(0)}$ via Lemma~\ref{lem:zeroth_suffice}, and can set $x' \gets x^{(0)}$.

To bound the runtime, note that applying Lemma~\ref{lem:three points} to each set of three coordinates corresponding to a consecutive pair of constraints takes $O(1)$ time, and $|S| = O(n)$ because of the following:
\begin{align*}
    |S| &\leq \sum_{\ell = 0}^k 2^{k-\ell} + 2\sum_{\ell=1}^k\sum_{m = 0}^{\ell-1} 2^{k-\ell} \leq 2^{k+1} + 2\sum_{\ell=1}^k \ell 2^{k-\ell}\\
    &\leq 2^{k+1} +2\sum_{\ell = 1}^{k} k 2^{k-\ell} - 2\sum_{\ell = 1}^{k} (k-\ell) 2^{k-\ell}\\
    &\leq 2^{k+1} + 2k2^{k} - 2(k-2)2^{k} \leq 2n+4n = O(n).
\end{align*}
\end{proof}

By combining Lemma~\ref{lem:round_def_smooth} with Corollary~\ref{cor:l_inf}, we have our main result of this section.

\begin{proposition}\label{prop:smCE}
Let $\eps \ge 0$. We can compute $x \in \xset$, an $\eps$-approximate minimizer to \eqref{eq:smce_empirical_appendix}, in time
\[O\Par{\frac{n\log(n)}{\eps}}.\]
Further, the objective value of $x$ in \eqref{eq:smce_empirical_appendix} is an $\eps$-additive approximation of $\smce(\hcD_n)$.
\end{proposition}
\begin{proof}
Observe that for $\tma$ defined in \eqref{eq:round_def_smooth}, we have $\norms{\tma}_{\infty \to \infty} = 2$ and $\nnz(\tma) = 4|S| = O(n)$. Therefore, Corollary~\ref{cor:l_inf} shows we can compute an $\eps$-approximate minimizer to
\[\min_{x \in [-1, 1]^n} c^\top x + \norm{\max\Par{\tma x - \tb, \0_{2|S|}}}_\infty\]
within the stated runtime. Finally, the definition of $\Round$ from Lemma~\ref{lem:round_def_smooth} shows that given this $\eps$-approximate minimizer, we can then produce an $\eps$-approximate minimizer to \eqref{eq:smce_empirical_appendix} in $O(n)$ time. The last claim in the lemma statement follows immediately from the definition of \eqref{eq:smce_empirical_appendix}.
\end{proof}

\subsection{Sufficiency and insufficiency of \texorpdfstring{$\SB$}{Sbase}}\label{ssec:sbase}

In this section, we give a brief discussion of an alternative strategy to that in Section~\ref{ssec:round_smooth}. Specifically, suppose we let $S$ in \eqref{eq:enforce_constraints_def} only consist of the pairs in $\SB$. We instead define $(\tma, \tb)$ as follows:
\begin{equation}\label{eq:simpler_def}
\begin{aligned}
\tma \in \R^{2|\SB| \times n} \text{ has } \tma_{(s, +):} \defeq (L + 1)\ma_{(s, +):},\; \tma_{(s, -):} \defeq (L + 1)\ma_{(s, -):} \text{ for all } s \in \SB, \\
\tb \in \R^{2|\SB|} \text{ has } \tb_{(s, +)} \defeq (L + 1)b_{(s, +)},\; \tb_{(s, -)} \defeq (L + 1)b_{(s, -)} \text{ for all } s \in \SB.
\end{aligned}
\end{equation}

Here, $L \defeq \lfloor\log_2(n - 1)\rfloor$ as in \eqref{eq:enforce_constraints_def}. In other words, $\tma, \tb$ take a subset of rows of $\ma, b$ and scale them up by $L + 1$. We first show that enforcing this simpler set of constraints yields a rounding procedure losing only a logarithmic factor in quality over the more complicated Lemma~\ref{lem:round_def_smooth}.

\begin{lemma}\label{lem:round_def_smooth_log}
Let $(\ma, b, c, \xset)$ be defined as in \eqref{eq:smce_empirical_appendix}, and let $(\tma, \tb)$ be defined as in \eqref{eq:enforce_constraints_def}, \eqref{eq:simpler_def}. There exists $\Round$, a $(\tma, \tb, \infty)$-inequality rounding procedure for $(\ma, b, c, \xset)$ running in $O(n)$ time.
\end{lemma}
\begin{proof}
For a fixed $x \in \xset$, let
\[\Delta \defeq \frac 1 {L + 1}\norm{\max\Par{\tma x - \tb, \0_{2|S|}}}_\infty,\]
so that $\Delta$ is the maximum violation of any Lipschitz constraint in $S$ at the start of the algorithm, since we have undone the scaling by $L + 1$. We claim we can produce $x' = \Round(x) \in \xset$ with $\ma x' \le b$ (i.e.\ $x'$ satisfies all of the Lipschitz constraints in $[n] \times [n]$), such that $\norm{x - x'}_\infty \le \delta(L + 1)$. The proof that $\Round$ is a $(\tma, \tb, \infty)$-inequality rounding procedure is then identical to Lemma~\ref{lem:round_def_smooth}.

To produce such $x'$, we again apply Lemma~\ref{lem:three points} to one layer of constraints at a time, producing a sequence $\{x^{(\ell)}\}_{\ell = 0}^{L + 1}$. Specifically, in place of the invariants in the proof of Lemma~\ref{lem:round_def_smooth}, we instead enforce the following invariants on $x^{(\ell)}$, for all $0 \le \ell \le L$.
\begin{enumerate}
    \item Every Lipschitz constraint $s$ in the $\ell^{\text{th}}$ layer of constraints is satisfied, i.e.\ $\ma_{s:} x \le b_s$. \label{item:row_fixed_2}
    \item $\norms{x^{(\ell)} - x^{(\ell + 1)}}_\infty \le \Delta(L + 1 - \ell)$.\label{item:inf_bound_2}
    \item Only coordinates of the form $j = i2^\ell + 1$ for odd $i \in \Z_{\ge 0}$ have $x^{(\ell + 1)}_j \neq x^{(\ell)}_j$. \label{item:sparse_move_2}
\end{enumerate}
The proof that Item~\ref{item:inf_bound_2} is inductively maintained replaces the use of Lemmas~\ref{lem:protect_constraints_1},~\ref{lem:protect_constraints_2} with the triangle inequality, since each constraint is originally violated by at most $\Delta$, and Lemma~\ref{lem:three points} moves $\ell^{\text{th}}$-layer constraints by at most $\Delta(L + 1 - \ell)$ via Item~\ref{item:inf_bound_2}. The rest of the proof is identical to Lemma~\ref{lem:round_def_smooth}.
\end{proof}

By plugging in Lemma~\ref{lem:round_def_smooth_log} into Corollary~\ref{cor:l_inf} instead of Lemma~\ref{lem:round_def_smooth}, we lose a $\log(n)$ factor in runtime, since $\norms{\tma}_{\infty \to \infty} = 2(L + 1) = O(\log(n))$. We next show this loss is inherent, if we only enforce $\SB$.

\begin{lemma}\label{lem:lowerbound_movement}
Let $L \in \N$, let $n = 2^L + 1$, and define $\ma, b$ as in \eqref{eq:smce_empirical_appendix}, and $\SB$ as in \eqref{eq:enforce_constraints_def}. There exists $x \in [-1, 1]^n$ and $\Delta \in [0, 1]$ such that, letting $[\ma x - b]_{\SB}$ denote the $2|\SB|$ coordinates of the vector $\ma x - b$ corresponding to elements of $\SB$,
\begin{gather*}\norm{\max\Par{[\ma x - b]_{\SB}, \0_{2|\SB|}}}_\infty = \Delta,\end{gather*}
but $\norms{\max([\ma x - b]_{\SB}, \0_{2|\SB|})}_\infty > 0$ for any $x' \in [-1, 1]^n$ with $\norms{x' - x}_\infty \le \frac{L\Delta} 2$.
\end{lemma}
\begin{proof}
Let $L \in \N$, $n = 2^L + 1$, and let $L\Delta \le 1$. We consider the following hard example:
\begin{gather*}x_j =  (L -\lceil\log_2(2^L-j+1) \rceil)\Delta \text{ for all } j\in [n-1]\text{ and } x_n = L\Delta,\\
v_j =  0 \text{ for all } j\in [n-1]\text{ and } v_n = L\Delta.\end{gather*}
For example, if $L = 3$ so $n = 9$, we have 
\[x_1 = \ldots = x_4 = 0,\; x_5 = x_6 = \Delta,\; x_7 = 2\Delta,\; \text{ and } x_8 = x_9 = 3\Delta.\]

We first show that none of the constraints is violated by more than $\Delta$ in the set $\SB$ for our construction. The $L^{\text{th}}$ layer is not violated because $x_n-x_1 = v_n-v_1$. Now, for the $\ell^{\text{th}}$ layer where $0 \le \ell < L$, we want to show that for any $i \in [2^{L - \ell}]$, the constraint $((i - 1)2^\ell + 1, i2^\ell + 1)$ is violated by at most $\Delta$. If $L = 2^{L - \ell}$, this is obvious because
\[\abs{x_n - x_{(i - 1)2^\ell + 1}} \leq v_n - v_{(i - 1)2^\ell + 1} = L\Delta.\]
Otherwise, because $|\lceil\log_2(2^L-(i - 1)2^\ell)\rceil-\lceil\log_2(2^L-i2^\ell)\rceil|\leq 1$  for $i < 2^{L - \ell}$, 
\[\abs{x_{i 2^\ell + 1} -x_{(i - 1)2^\ell + 1}}\leq \Delta = \Delta + v_{i2^\ell + 1} - v_{(i - 1)2^\ell + 1}.\]
Finally, if $x'$ satisfies all Lipschitz constraints, $x'_1 = x'_{2^L}$, so one of $x_1$ or $x_{2^L}$ must move by $\frac{L\Delta}{2}$.
\iffalse
Notice in the construction above only the following set of $\log (n-1)$ constraints to violating by $\Delta$ each: 
\begin{align*}        
S_{\text{hard}}=&\Par{[n] \times [n]} \cap \bigcup_{\ell = 0}^{L-1}\Brace{\Par{2^L - 2^{L-\ell}+ 1, 2^L - 2^{L-\ell-1} + 1} }
\end{align*} 

Further, let's consider these $\lfloor\log ((n-1))/2\rfloor^{\text{th}}$ constraints in set $\SH$, denoted by $x_j - x_k = v_j-v_k+\Delta$. To fix this constraint, we either have $x_j-y_j \geq \Delta/2$, move $x_j$ to left by $\Delta/2$, or $y_k-x_k\geq\Delta/2$, move $x_ik$ to the right by at least $\Delta/2$. Hence we have either $y_k - x_1 =\Delta\lfloor\log ((n-1))/2\rfloor$ or $x_{n-1}-y_j = \Delta\lfloor\lfloor\log ((n-1))/2\rfloor$ which requires $y_1 - x_1\geq  \Delta\lfloor\lfloor\log ((n-1))/2\rfloor$, $x_1$ move to the right or $x_{n-1} - y_{n-1}\geq  \Delta\lfloor\lfloor\log ((n-1))/2\rfloor$, $x_{n-1}$ move to the left.
\fi
\end{proof}

\iffalse

\begin{remark}
    The first idea we had to formulate this optimizing problem is using $2n$ constraints for each $1\leq j\leq n-1$, $\abs{x_{j+1}-x_{j}}\leq v_{j+1}-v_{j}$. However, for example, if we have $x_1, \dots x_4$, and $x_{j+1}-x_{j} = v_{j+1}-v_{j} + \eps$ for $1\leq j\leq 3$, there is not a way to fix the constraint violations by moving any $x_j$ by at most $\eps$. The idea is that if we want to fix $x_3-x_2$, we need to either increase $x_2$ or decrease $x_3$ and make it takes more than moving $x_1$ or $x_4$ more than $\eps$ to fix $x_2-x_1$ or $x_4-x_3$. So we need to formulate a problem with more than $2n$ constraints.
\end{remark}
\fi
